# Supplementary material for: From Realizability Modulo Theories to Synthesis Modulo Theories Part 1: Dynamic approach
Source: arXiv:2310.07904 source file (2023-10-11)
Supplement: Supplementary file 1 [file 7-appendix.tex]

\section{Appendix: complete example}

We use the modified running example $\phiT'$ to show that a synthetised full $\Theo$-controller always 
has the opportunity to provide with outputs that do not violate the specification, 
(since the Boolean controller is realizable). 
Note that a valid (positional) strategy of the system is to always play $y=2$; 
which is equivalent to saying that a synthesised machine could have been a constant function $y=f(\barX)=2$. 
In this particular trace execution (see Fig.~\ref{figSim}), the system has always played $y=2$ 
(preserving satisfaction) except for the first timestep.
We show that the $\Theo$-controller can always play $y=2$ infinitely many often and 
we also show that in some timesteps other outputs are also possible.
Note that we use the notation $c_i$ to indicate choice $i$; e.g., 
$c_0 \equiv s_{012}$, $c_1 \equiv \Cone$, etc,
where $s_{012}$ means $s_0 \wedge s_1 \wedge s_2$, 
$\Cone$ means $s_0 \wedge s_1 \wedge \neg s_2$, etc.
%Fig.~\ref{figAutomataRunningEx} shows the automata synthetised of $\phiT'$ by Strix. 
%
%\begin{figure}[t!]
%  \centering
%  \includegraphics[scale=0.25]{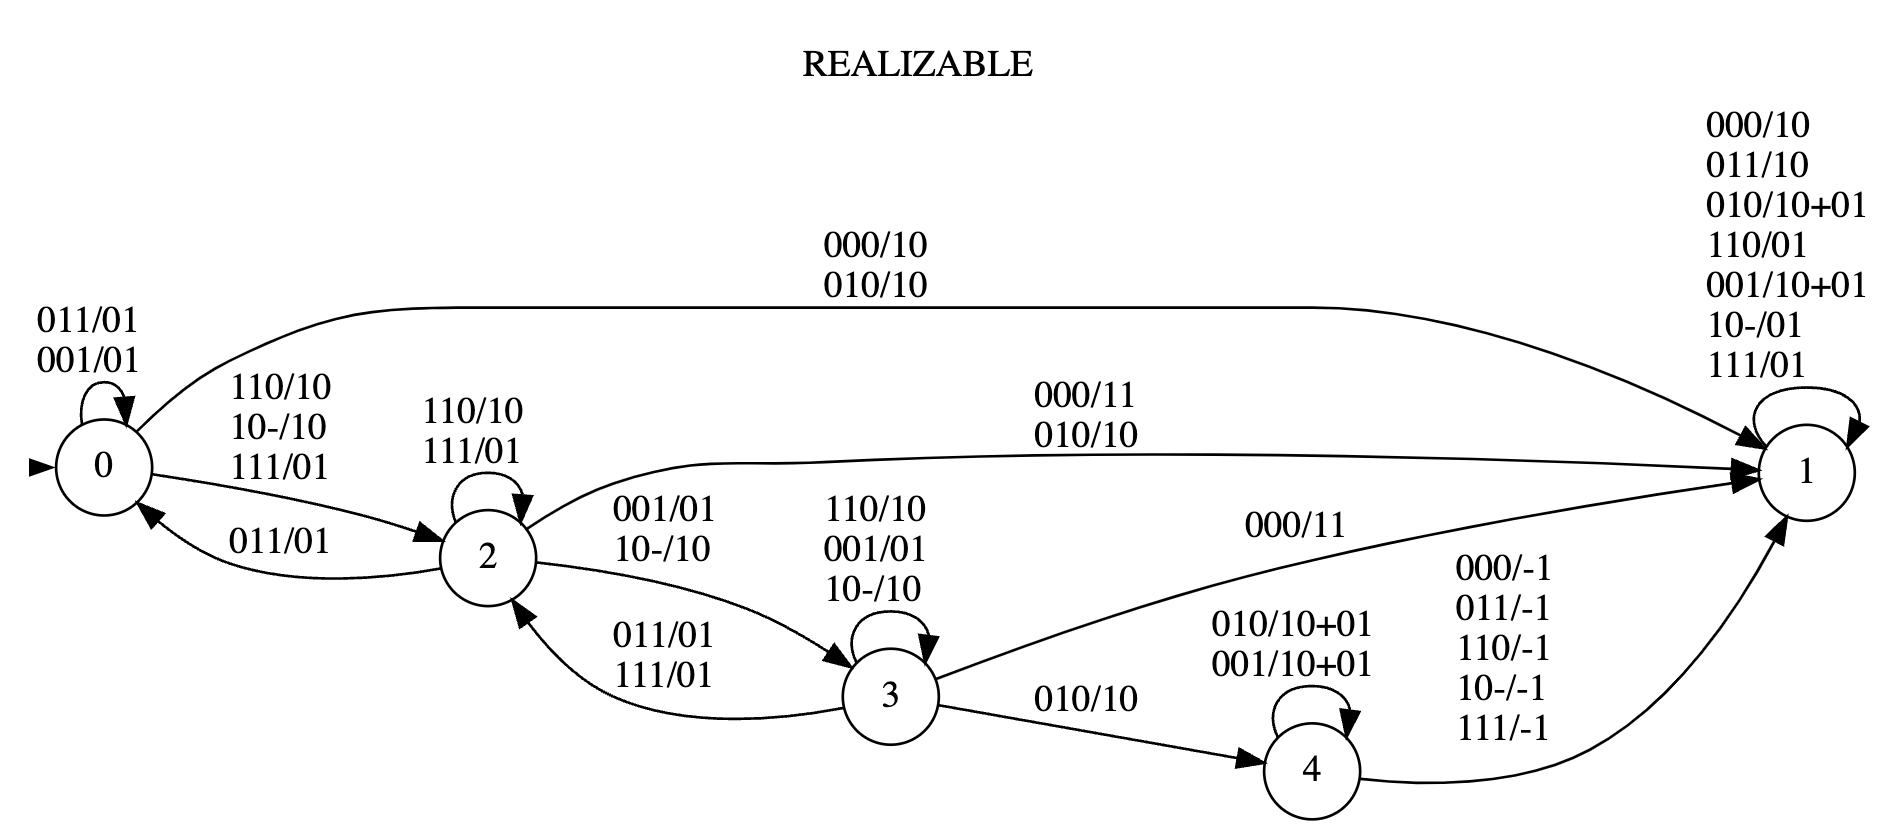}
%  \caption{Strix automata corresponding to $\phiT'$.}
%  \label{figAutomataRunningEx}
%\end{figure}

\begin{figure} %[htbp]
\centerline{\includegraphics[scale=0.3]{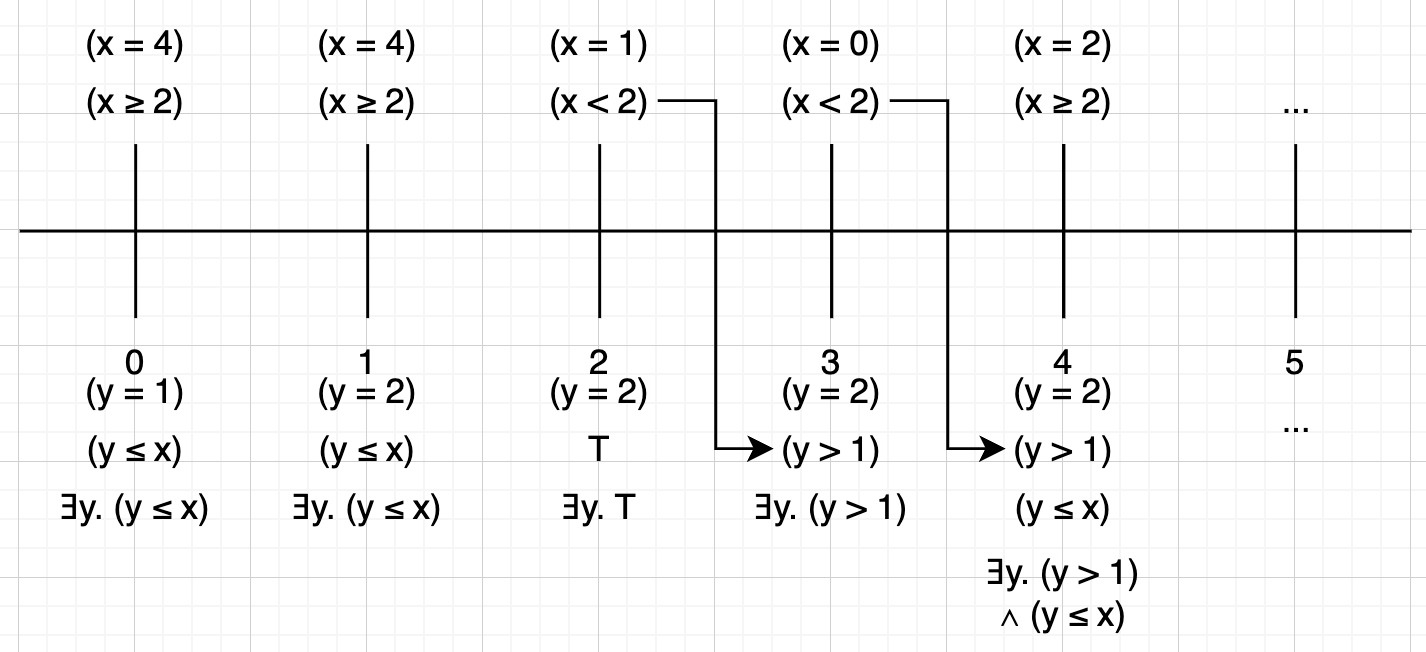}}
\caption{Simulation of 5 steps, where we can see what values the environment chooses (and which is the predicate that this choice satisfies), together with the values that the system chooses according to the restrictions (of the current timestep or/and of the previous timestep).}
\label{figSim}
\end{figure}

\subsubsection{Step 1: Environment forces instant response.}

Let $x=4$, which holds $(x \geq 2)$ and forces constraint $(y \leq x)$. We are in partition $e_1$, which implies choices $\{ c_4, c_5, c_6\}$.
Thus, the system can choose $c_6$ to imitate the $\overline{y}=[y=1]$ of Fig.~\ref{figSim}. Further details are as follows:
\begin{enumerate}
    \item $\exists \overline{y} \textit{. }c_4(\overline{y},\overline{x})$, with fixed $\overline{x}_{\mathcal{T}}=[x=4]$.
    \begin{itemize}
        \item $\mathbb{B}:\neg s_0 \wedge s_1 \wedge s_2$ 
        \item $\mathcal{T}: (x \geq 2) \wedge (y>1) \wedge (y \leq x)$ \\
        $(4 \geq 2)^{\checkmark} \wedge (y>1) \wedge (y \leq 4),$
    \end{itemize}
    where the \checkmark denotes that a ground predicate holds, because it is the environment decision itself.
    
    Thus, we have a finite set of models $m(\overline{y})=\{2,3,4\}.$ Take, e.g., the \textit{least}: i.e., $\overline{y}=[y=2]$, which holds the $(y \leq x)$ constraint of the specification. Thus, in this step, $c_4$ is not violating the specification; i.e., the system in $\mathbb{B}$ will potentially choose it in these plays. 
    Note that, particularly $c_4$, can always be chosen.
    \item $\exists \overline{y} \textit{. }c_5(\overline{y},\overline{x})$.
    \begin{itemize}
        \item $\mathbb{B}:\neg s_0 \wedge s_1 \wedge \neg s_2$ 
        \item $\mathcal{T}: (x \geq 2) \wedge (y>1) \wedge (y > x)$ \\
        $(4 \geq 2)^{\checkmark} \wedge (y>1) \wedge (y > 4)$
    \end{itemize}
    Thus, we have infinite models $m(\overline{y})=\{5,6,7,...\}.$ Take least, i.e., $\overline{y}=[y=5]$, which does not hold the $(y \leq x)$ constraint of the specification. Thus, in this step, $c_5$ is violating the specification; i.e., the system in $\mathbb{B}$ will never choose it in these plays. Note that, indeed, $c_5$ can never be chosen without violating the specification.
    \item $\exists \overline{y} \textit{. }c_6(\overline{y},\overline{x})$.
    \begin{itemize}
        \item $\mathbb{B}:\neg s_0 \wedge \neg s_1 \wedge s_2$ 
        \item $\mathcal{T}: (x \geq 2) \wedge (y \leq 1) \wedge (y \leq x)$ \\
        $(4 \geq 2)^{\checkmark} \wedge (y \leq 1) \wedge (y \leq 4)$
    \end{itemize}
    Thus, we have infinite models $m(\overline{y})=\{1,0,-1,...\}.$ Take, e.g., greatest: $\overline{y}=[y=1]$, which holds the $(y \leq x)$ constraint of the specification. Thus, in this step, $c_6$ is not violating the specification; however, note that $c_6$ is not like $c_4$ in the sense that it cannot always be chosen to not violate the specification (see step 5). 
    
    Also, note that the constraint $(y \leq 1)$ created by the Boolean abstraction algorithm is harder than the only constraint $(y\leq x)$ of the specification; thus, this suggests that the current algorithm of  Boolean abstraction is \textit{too exigent} in the sense that it considers more cases than necessary. %This is an example of why (bounded) temporality should be used in (new) Boolean abstraction algorithms.
\end{enumerate}

\subsubsection{Step 2: Environment repeats the strategy.}

Environment plays the same and (see Fig.~\ref{figSim}) responds with $\barY=[y=2]$, so the system has to choose $c_4$ to imitate it. 

\subsubsection{Step 3: Environment changes its mind.}

Let $x=1$, which holds $(x < 2)$ and forces constraint $\Next(y > 1)$, whereas no constraint is further for the current timestep. We are in partition $e_0$, which implies choices $\{c_1, c_2\}$.
The system can choose $c_1$ to imitate the $\overline{y}=[y=2]$ of Fig.~\ref{figSim} (which is the positional strategy). Note that this step has restriction $\top$ (i.e., no one), because it has forced a constraint only for the next timestep.
Further details are as follows:
\begin{enumerate}
    \item $\exists \overline{y} \textit{. }c_1(\overline{y},\overline{x})$, with fixed $\overline{x}_{\mathcal{T}}=[x=1]$.
    \begin{itemize}
        \item $\mathbb{B}: s_0 \wedge s_1 \wedge \neg s_2$ 
        \item $\mathcal{T}: (x < 2) \wedge (y>1) \wedge (y > x)$ \\
        $(1 < 2)^{\checkmark} \wedge (y>1) \wedge (y > 1)$
    \end{itemize}
    Thus, we have infinite models $m(\overline{y})=\{2,3,4,...\}.$ Take least, i.e., $\overline{y}=[y=2]$, which holds the $\top$ constraint of the specification. Thus, in this step, $c_1$ is winning.
    Note that, particularly $c_1$, can always be chosen to hold the specification. Also, note that both $(y>1)$ and $(y > x)$ are restrictions harder than $\top$.
    \item $\exists \overline{y} \textit{. }c_2(\overline{y},\overline{x})$.
    \begin{itemize}
        \item $\mathbb{B}: s_0 \wedge \neg s_1 \wedge s_2$ 
        \item $\mathcal{T}: (x < 2) \wedge (y \leq 1) \wedge (y \leq x)$ \\
        $(1 < 2)^{\checkmark} \wedge (y \leq 1) \wedge (y \leq 1)$
    \end{itemize}
    Thus, we have infinite models $m(\overline{y})=\{1,0,-1,...\}.$ Take greatest, i.e., $\overline{y}=[y=3]$, which holds the $\top$ constraint of the specification. Thus, in this step, $c_2$ is winning; however, note that choosing $c_2$ (unlike $c_1$) does not always guarantee to hold the specification (see step 4). 
    Again, note that both $(y \leq 1)$ and $(y \leq x)$ are restrictions harder than $\top$.
\end{enumerate}

\subsubsection{Step 4: Environment prepares its trap.}

Let $x=0$, which holds $(x < 2)$ and forces constraint $\Next(y > 1)$, and take into account that the system has constraint $(y > 1)$ forced by the previous timestep. We are in partition $e_0$, which implies, again, choices $\{c_1, c_2\}$.
%
%The system can choose $c_1$ to imitate the $\overline{y}=[y=2]$ of Fig.~\ref{figSim} (which is the positional strategy). 
%
Further details are as follows:
\begin{enumerate}
    \item $\exists \overline{y} \textit{. }c_1(\overline{y},\overline{x})$, with fixed $\overline{x}_{\mathcal{T}}=[x=0]$.
    \begin{itemize}
        \item $\mathbb{B}: s_0 \wedge s_1 \wedge \neg s_2$ 
        \item $\mathcal{T}: (x < 2) \wedge (y>1) \wedge (y > x)$ \\
        $(0 < 2)^{\checkmark} \wedge (y>1) \wedge (y > 0)$
    \end{itemize}
    Thus, we have infinite models $m(\overline{y})=\{2,3,...\}.$ Take least, i.e., $\overline{y}=[y=2]$, which holds the $\top$ constraint of the specification.
    \item $\exists \overline{y} \textit{. }c_2(\overline{y},\overline{x})$.
    \begin{itemize}
        \item $\mathbb{B}: s_0 \wedge \neg s_1 \wedge s_2$ 
        \item $\mathcal{T}: (x < 2) \wedge (y \leq 1) \wedge (y \leq x)$ \\
        $(1 < 2)^{\checkmark} \wedge (y \leq 1) \wedge (y \leq 0)$
    \end{itemize}
    Thus, we have infinite models $m(\overline{y})=\{0,-1,-2...\}$. However, no one of these holds the constraint $(y>1)$ that was forced from previous timestep; thus, the system will never choose $c_2$ in this play. %This is why $c_2$ is not an \textit{statically winning choice}. 
\end{enumerate}

\subsubsection{Step 5: Environment strikes back!}

Let $x=2$, which holds $(x \geq 2)$ and forces constraint $(y \leq x)$. 
Also, note that the system has constraint $(y>1)$ from previous timestep. 
We are in partition $e_1$, which implies choices $\{ c_4, c_5, c_6\}$.
The system can (only) choose $c_4$ to imitate the $\overline{y}=[y=1]$ of Fig.~\ref{figSim}.
Further details are as follows:
\begin{enumerate}
    \item $\exists \overline{y} \textit{. }c_4(\overline{y},\overline{x})$, with fixed $\overline{x}_{\mathcal{T}}=[x=4]$.
    \begin{itemize}
        \item $\mathbb{B}:\neg s_0 \wedge s_1 \wedge s_2$ 
        \item $\mathcal{T}: (2 \geq 2) \wedge (y>1) \wedge (y \leq 2)$ \\
        $(4 \geq 2)^{\checkmark} \wedge (y>1) \wedge (y \leq 4)$
    \end{itemize}
    Thus, we have a finite model $m(\overline{y})=\{2\}.$ Take, $\overline{y}=[y=2]$, which holds the $(y \leq x)$ constraint of the specification and also the previously forced constraint $(y>1)$. Thus, $c_4$ is not violating the specification.
    \item We skip 
    %$c_5^{(P)}$, 
    $c_5$, since it will not be chosen, as remarked in step 1.
    \item $\exists \overline{y} \textit{. }c_6(\overline{y},\overline{x})$.
    \begin{itemize}
        \item $\mathbb{B}:\neg s_0 \wedge \neg s_1 \wedge s_2$ 
        \item $\mathcal{T}: (x \geq 2) \wedge (y \leq 1) \wedge (y \leq x)$ \\
        $(2 \geq 2)^{\checkmark} \wedge (y \leq 1) \wedge (y \leq 2)$
    \end{itemize}
    Thus, we have infinite models $m(\overline{y})=\{1,0,-1,...\}.$ Take greatest: $\overline{y}=[y=1]$, which holds the $(y \leq x)$ constraint of the specification. However, this model does not also hold the previously forced predicate $(y>1)$; thus, $c_6$ is violating the specification in this step, and the system will not choose it.
\end{enumerate}

Fig.~\ref{figSimTZTB} summarizes all the steps above and the relationship between the Boolean game and the theory game.

\begin{figure} %[htbp]
\centerline{\includegraphics[scale=0.3]{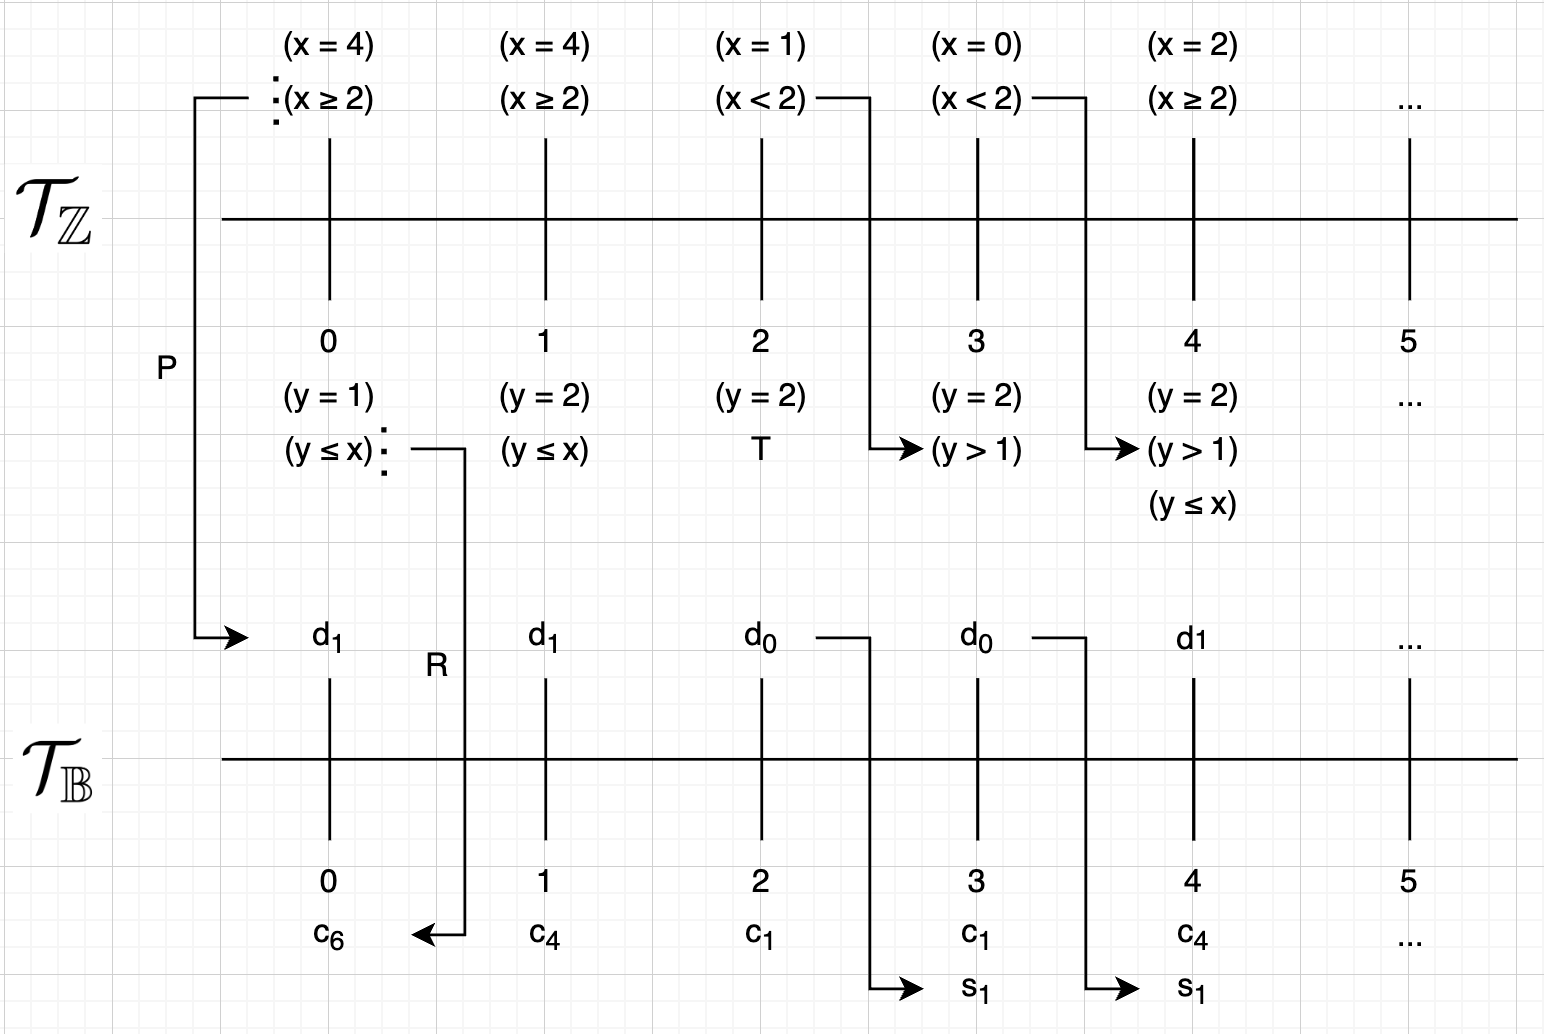}}
\caption{
    We can see the $\ThZ$ play above and the equi-satisfied $\mathcal{T}_{\Boolbb}$ play below. 
    The P-labelled arrow between $(x \geq 2)$ and $d_1$ means that 
    $e_1$ is the \textit{decision} of the environment
    %$e_1$ or $e_2$ is the \textit{decision} of the environment 
    %(i.e., the partition $e_1 \cup e_2$); 
    which represents all $x$ such that $(x \geq 2)$  holds (resp. $(x<2)$ with $d_0$). 
    The R-labelled arrow between $(y \leq x)$ and $c_6$ means $\exists y \suchThat c_6$, where $c_6 \equiv (\neg s_0 \wedge \neg s_1 \wedge s_2)$; and, resp. $(y \leq x)$ with $\exists y \suchThat c_4$, $\top$ with $\exists y \suchThat c_1$, $(y > 1)$ with $\exists y \suchThat c_1$ and $((y>1) \wedge (y \leq x))$ with $\exists y \suchThat c_6$. Note that, e.g., $c_4$ in the step $0$ and $c_2$ in the step $2$ were also possible choices of the system that the Boolean controller has decided not to play.}
\label{figSimTZTB}
\end{figure}
