# Supplementary material for: From Realizability Modulo Theories to Synthesis Modulo Theories Part 1: Dynamic approach
Source: arXiv:2310.07904 source file (2023-10-11)
Supplement: Supplementary file 2 [file appendix.tex]

\section{Appendix}

//We show, among others, preprocessing times necessary; i.e.,  BA+synth+composition times
